# Supplementary material for: Clustering a Mixture of Gaussians with Unknown Covariance
Source: arXiv:2110.01602 source file (2021-11-29)
Supplement: Supplementary file 1 [file appendix-gap-landscape.tex]

\section{More about Section \ref{sec-gap}}\label{sec-gap-appendix}
